# Supplementary material for: Dynamic relaxation oscillations in a nonlinearly driven quartz crystal
Source: arXiv:1509.03096 source file (2015-09-10)
Supplement: Supplementary file 1 [file Houri15-SI.pdf]

# Supplemental Material to:
# Dynamic relaxation oscillations in a nonlinearly driven quartz crystal

S. Houri,[1] M. J. Geuze,[1] and W. J. Venstra[1,*]

[1] *Kavli Institute of Nanoscience, Delft University of Technology, Lorentzweg 1, 2628 CJ Delft, The Netherlands*

*Electronic address: `w.j.venstra@tudelft.nl`

**Description of the electronic circuit**

Fiure S1 shows a schematic of the electronic circuit. The driving signal, generated by the lock-in amplifier, is amplified to deliver about $I_p = 200\,mA$ at $V_P = 10\,V$ at a bandwidth up to 14 MHz. To this end, a Mini-Circuits amplifier (U5, ZHL-32A), an opamp (U1, LT1363) and buffers (U2 and U3, BUF634, placed in parallel to increase the output current) are used. An RC-filter in the feedback path (R1,C1) ensures a stable unity gain and suppresses high-frequency oscillations. The current is measured using resistor R4, and fed into the lock-in via U4. This current detection circuit was simulated in LTspice IV using component models provided by the manufacturer. Figure S2 shows the frequency response of the voltage presented to the lock-in input, referred to the voltage on the crystal. The simulation predicts an almost flat amplitude response over the range of interest, up to about 30 MHz.

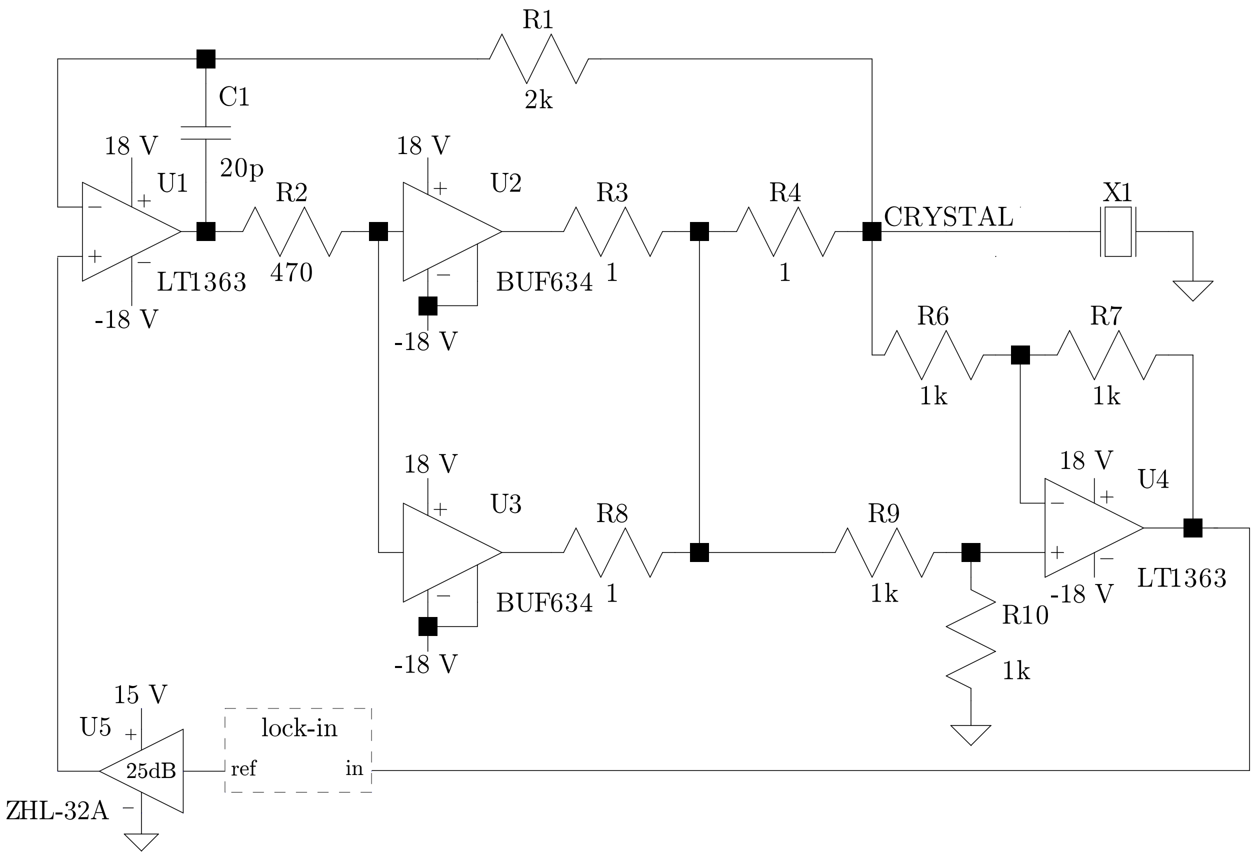


FIG. S1: Schematic of the measurement circuit. An AT-cut crystal is used, manufacturer number HC49U-4.608-20-50-60-30-ATF, with a parallel resonance frequency at 4.608 MHz.

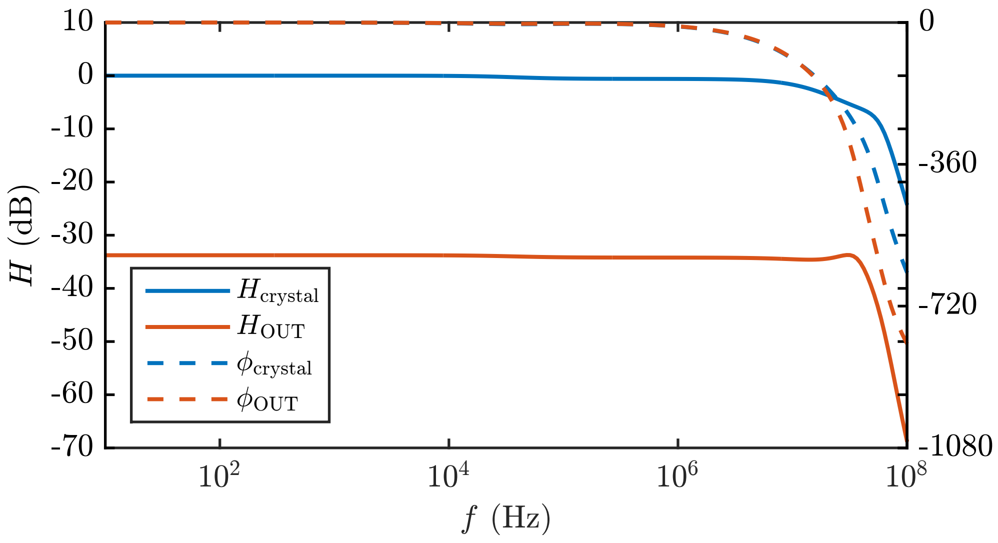


FIG. S2: Frequency response of the detection circuit as simulated in LTspice.

The electrical impedance of the crystal strongly depends on the amplitude of its motion. In order not to skew the amplitude-frequency dependence measurements, the circuit should be capable of driving a strongly varying load at a constant voltage amplitude. To characterize the circuit under load, the output voltage is simulated as a function of the resistive load in LTspice. In the simulation, the crystal is substituted by a parallel resistance and capacitance. Figure S3 shows the result: the response of the circuit is flat (red solid line), compared to a power amplifier with a $50\,\Omega$ output impedance (blue solid line). The figure also shows the measurements, which are within 2% of the predicted values for $\mathrm{R} \geq 18\,\Omega$. For a higher driving voltage and a lower load resistance, the maximum output current of the buffer is approached and the error increases. In the present experiments however, the load resistance $\mathrm{R} > 20\,\Omega$ and the maximum voltage is $\mathrm{V_p} = 2.5\,\mathrm{V}$. In this regime, the designed driving circuit is a stable voltage source.

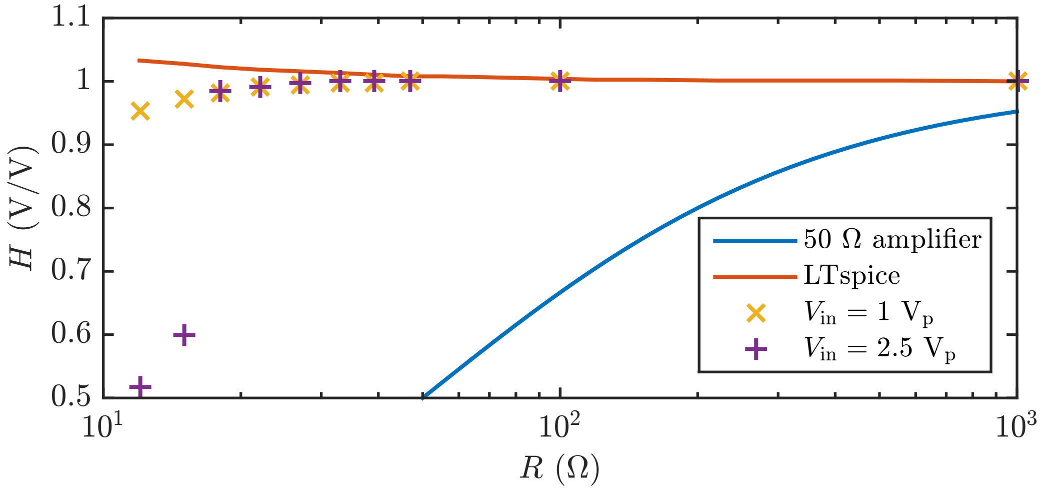


FIG. S3: Response as a function of the resistive load. Blue solid line: calculated response of a standard amplifier with $50\,\Omega$ output impedance. Red solid line: calculated response of the design of Fig. S1. Crosses: measured response of the implemented circuit.
